# Supplementary material for: Identifying and Correcting Label Bias in Machine Learning
Source: arXiv:1901.04966 source file (2019-01-15)
Supplement: Supplementary file 1 [file AdditionalFairness.tex]

\section{Fairness Experiments with Additional Baselines}

\subsection{Additional Baselines}

We now compare against additional Lagrangian baselines recommended by \cite{cotter2018optimization}, which gave a thorough analysis of Lagrangian-based methods and their application to fair machine learning:
\begin{itemize}
    \item {\bf Hinge Lagr.} This was the Lagrangian baseline of \cite{eban2017scalable} used in Table~\ref{tab:experiments} which proceeds by performing a Hinge relaxation of the fairness constraints to make the Lagrangian differentiable so that it can be trained by gradient-based methods.
    \item {\bf 0/1 Lagr.} This was the method recommended by \cite{cotter2018optimization} which they call "0/1 Best External." It proceeds by playing a two-player game where one player minimizes the Hinge-relaxed Lagrangian but the other player enforces fairness by learning the Lagrange multipliers based on the original fairness constraint (rather than a Hinge relaxation). This leads to a non-zero-sum two-player game and each player proceeds by alternating performing SGD on their respective objectives. Then at the end, a heuristic is used to choose the "best" iterate based on the fairness and accuracy on the training set.
    We tune the hyperparameters (i.e. fairness slack and number of iterations) the same as in the Hinge Lagr. baseline.
    \item  {\bf 0/1 Lagr. Full} This is the same as the previous, but instead of each player taking a stochastic gradient descent step, each player takes a full gradient step computed over the entire training set.
\end{itemize}
We note that \cite{cotter2018optimization} also recommend another baseline which learns a randomized classifier, but the scope of our work deals with deterministic classifiers.

\subsection{Results}
We show results by fairness metric: Demographic Parity (Table~\ref{tab:experiments_demparity}), Disparate Impact (Table~\ref{tab:experiments_disparate}), Equal Opportunity (Table~\ref{tab:experiments_equalopp}), and Equalized Odds (Table~\ref{tab:experiments_equalodds}).

We see that our method outperforms the state of art for Demographic Parity and performs competitively with the Lagrangian methods on the other notions of fairness despite being a simpler approach.

\begin{table*}
\setlength{\tabcolsep}{5pt}
\begin{center}
  \caption{{\bf Additional Demographic Parity Results}}
  \label{tab:experiments_demparity}
  \begin{tabular}{|l|r|r|r|r|r|r|}
 \hline
Dataset & Unconstrained & Calibration &  Hinge Lagr. & 0/1 Lagr. &  0/1 Lagr. Full & Our Method \\
\hline
Bank Err. & 9.41\% & 9.7\% &	10.46\% &	9.65\% &	11.22\% &	9.63\% \\
Bank Vio.  & 0.0349	 & 0.0068 &	0.0126 &	0.018	& 0.0068 & {\bf  0.0056} \\
\hline
COMPAS Err. & 31.49\% & 	32.53\% & 	40.16\% & 	38.02\% & 	39.69\% & 	35.44\%  \\
COMPAS Vio.&  0.2045 &	0.0201&	0.0495 &	0.0462 &	0.0477 &	{\bf 0.0155} \\
\hline
Communities Err.&  11.62\% & 	32.06\% & 	28.46\% & 	24.45\% & 	23.84\% & 	30.06\% \\
Communities Vio. & 0.4211 &	0.0653	& 0.0519	& 0.1204 &	0.1538 &	{\bf 0.0107} \\
\hline
German Stat. Err.  & 24.85\% & 	24.85\% & 	25.45\% & 	27.27\% & 	27.88\% & 	25.15\%  \\
German Stat. Vio. & 0.0766 &	0.0346 &	0.041 &	0.0681 &	0.0802 &	{\bf 0.0137} \\
\hline
Adult Err.   & 14.15\% & 	16.6\% & 	20.47\% & 	19.57\% & 	19.71\% & 	16.51\%  \\
Adult Vio. & 0.1173	& 0.0129&	0.0198 &	0.0215 &	0.0277 &	{\bf 0.0037} \\
\hline
\end{tabular}
\end{center}
\end{table*}

\begin{table*}
\setlength{\tabcolsep}{5pt}
\begin{center}
  \caption{{\bf Additional Disparate Impact Results}}
  \label{tab:experiments_disparate}
  \begin{tabular}{|l|r|r|r|r|r|}
 \hline
Dataset & Unconstrained  &  Hinge Lagr. & 0/1 Lagr. &  0/1 Lagr. Full & Our Method \\
\hline
Bank Err. & 9.41\% &		10.44\% &	9.63\% &	9.94\% &	9.89\%  \\
Bank Vio.  & 0.0304	 &	0.0135 &	0.0179 &	0.0169 &	{\bf 0.0063} \\
\hline
COMPAS Err. & 31.21\% &		40.35\% &	38.97\% &	38.49\% &	42.64\% \\
COMPAS Vio.& 0.1362	 &	0.0499 &	0.0553	 & 0.0525 &	 {\bf 0.0256} \\
\hline
Communities Err.& 14.83\% &		28.26\% &	24.84\% &	25.05\% &	30.26\%  \\
Communities Vio. & 0.396	 &	0.0557 &	0.113 &	0.1224 &	{\bf 0.0073} \\
\hline
German Stat. Err.  & 24.85\% &		26.67\% &	25.45\% &	24.54\% &	25.15\%   \\
German Stat. Vio. & 0.0608 &	{\bf 0.0139} &	0.0167 &	0.0651 &	0.0156 \\
\hline
Adult Err.   & 14.19\% &		20.48\% &	19.76\% &	18.3\% &	17.37\%  \\
Adult Vio. &  0.1108 &	{\bf 0.0199} &	0.0233	& 0.0331	& 0.0334 \\
\hline
\end{tabular}
\end{center}
\end{table*}

\begin{table*}
\setlength{\tabcolsep}{5pt}
\begin{center}
  \caption{{\bf Additional Equal Opportunity Results}}
  \label{tab:experiments_equalopp}
  \begin{tabular}{|l|r|r|r|r|r|r|}
 \hline
Dataset & Unconstrained & Calibration &  Hinge Lagr. & 0/1 Lagr. &  0/1 Lagr. Full & Our Method \\
\hline
Bank Err. & 9.41\% &	9.55\% &	9.86\% &	9.64\% &	10.76\% &	9.48\% \\
Bank Vio.  & 0.1452 &	0.0506 &	0.1237 &	0.1061 &	0.1021 &	{\bf 0.0431} \\
\hline
COMPAS Err. & 31.49\% &	31.63\% &	36.92\% &	41.78\% &	38.59\% &	33.63\%  \\
COMPAS Vio.&  0.2373 &	{\bf 0.0256} &	0.1141 &	0.0411 &	0.092 &	0.0774 \\
\hline
Communities Err.&  11.62\% &	17.64\% &	28.45\% &	24.65\% &	26.65\% &	26.85\%  \\
Communities Vio. & 0.5513 & {\bf 	0.0584} &	0.0897 &	0.2115 &	0.1474 &	0.0833 \\
\hline
German Stat. Err.  & 24.85\% &	24.54\% &	27.27\% &	24.85\% &	24.54\% &	25.45\%  \\
German Stat. Vio. & 0.112 &	0.0922 &	0.0757 &	0.2032 &	0.096 &	{\bf 0.0662} \\
\hline
Adult Err.   & 14.15\% &	14.43\% &	19.67\% &	18.9\% &	17.95\% &	14.46\% \\
Adult Vio. & 0.1195 &	0.017 &	0.0374	& {\bf 0.0055} &	0.0099 &	0.0092\\
\hline
\end{tabular}
\end{center}
\end{table*}

\begin{table*}
\setlength{\tabcolsep}{5pt}
\begin{center}
  \caption{{\bf Additional Equalized Odds Results}}
  \label{tab:experiments_equalodds}
  \begin{tabular}{|l|r|r|r|r|r|}
 \hline
Dataset & Unconstrained  &  Hinge Lagr. & 0/1 Lagr. &  0/1 Lagr. Full & Our Method \\
\hline
Bank Err. &  9.41\% &		9.61\% &	9.66\% &	9.99\% &	9.5\%  \\
Bank Vio.  &  0.1452 &		0.0879 &	0.1093 &	0.1214 &	{\bf 0.0376} \\
\hline
COMPAS Err. & 31.49\% &		42.69\% &	42.35\% &	43.4\% &	35.06\%  \\
COMPAS Vio.& 0.2373	 &	0.0566 &	0.0576 &	{\bf 0.0477} &	0.0663 \\
\hline
Communities Err.& 11.62\% &		28.46\% &	23.84\% &	21.84\% &	26.65\%  \\
Communities Vio. & 0.5513 &		0.0962 &	0.2435 &	0.3205 &	{\bf 0.0769} \\
\hline
German Stat. Err.  & 24.85\%	&	27.57\% &	25.45\%	& 27.88\% 	& 25.45\%  \\
German Stat. Vio. & 0.112	 &	{\bf 0.0468} &	0.0919 &	0.074 &	0.1099 \\
\hline
Adult Err.   & 14.15\%	&	19.04\%  &	18.9\% &	18.13\% &	14.58\%   \\
Adult Vio. & 0.1195	&	0.016 &	{\bf 0.0156} &	0.0204 &	0.0221 \\
\hline
\end{tabular}
\end{center}
\end{table*}
